# Supplementary material for: Bayesian autoencoders for data-driven discovery of coordinates, governing equations and fundamental constants
Source: arXiv:2211.10575 source file (2022-11-19)
Supplement: Supplementary file 1 [file supp.tex]

\section{Network Architecture and Training}

\subsection{Network architecture}\label{sec:si_architecture}
The autoencoder network consists of a series of fully-connected layers. Each layer has an associated weight matrix $\Wv$ and bias vector $\bv$. We use sigmoid activation functions $f(x) = 1/(1+\exp(-x))$, which are applied at all layers of the network, except for the last layer of the encoder and the last layer of the decoder. Other choices of activation function, such as rectified linear units and exponential linear units, may also be used and appear to achieve similar results.

\subsection{Loss function}\label{sec:si_loss_function}
The loss function used in training is a weighted sum of four terms: autoencoder reconstruction $\Lrecon$, SINDy prediction on the input variables $\Lsindyx$, SINDy prediction on the encoder variables $\Lsindyz$, and SINDy coefficient regularization $\Lreg$. For a data set with $m$ input samples, each loss is explicitly defined as follows:
\begin{subequations}
\begin{align}
  \Lrecon &= \frac{1}{m} \sum_{i=1}^m \left\| \xv_i - \psi(\varphi(\xv_i))\right\|_2^2 \\
  \Lsindyx  &= \frac{1}{m} \sum_{i=1}^m \left\|\dot{\xv}_i - \left(\nabla_\zv\psi(\varphi(\xv_i))\right)\left(\Thetav(\varphi(\xv_i)^T)\Xiv\right)\right\|_2^2 \\
  \Lsindyz &= \frac{1}{m} \sum_{i=1}^m \left\|\nabla_\xv\varphi(\xv_i)\dot{\xv}_i - \Thetav(\varphi(\xv_i)^T)\Xiv\right\|_2^2 \\
  \Lreg &= \frac{1}{pd} \left\| \Xiv \right\|_1.
\end{align}
\end{subequations}
The total loss function is
\begin{equation}
  \Lrecon + \lambda_1 \Lsindyx + \lambda_2 \Lsindyz + \lambda_3 \Lreg.
\end{equation}
$\Lrecon$ ensures that the autoencoder can accurately reconstruct the data from the intrinsic coordinates. $\Lsindyx$ and $\Lsindyz$ ensure that the discovered SINDy model captures the dynamics of the system by ensuring that the model can predict the derivatives from the data. $\Lreg$ promotes sparsity of the coefficients in the SINDy model.

\subsection{Computing derivatives}\label{sec:computing_gradients}
Computing the derivatives of the encoder variables requires propagating derivatives through the network. Our network makes use of an activation function $f(\cdot)$ that operates elementwise. Given an input $\xv$, we define the pre-activation values at the $j$th encoder layer as
\begin{equation}
   % \lv_i = f(\lv_{i-1}\Wv_i + \bv_i).
   \lv_j = f(\lv_{j-1})\Wv_j + \bv_j.
\end{equation}
The first layer applies the weights and biases directly to the input so that
\begin{equation}
  \lv_0 = \xv \Wv_0 + \bv_0.
\end{equation}
The activation function is not applied to the last layer, so for an encoder with $L$ hidden layers the autoencoder variables are defined as
\begin{equation}
  % \zv = f\left(f\left(\cdots \left(f(\xv) \Wv_0 + \bv_0 \right)\cdots\right)\Wv_{n-1} + \bv_{n-1}\right)\Wv_n + \bv_n
  % \zv = f\left(\cdots f\left(\xv \Wv_1 + \bv_1 \right) + \bv_1 \cdots\right)\Wv_n + \bv_n
  \zv = f(\lv_{L-1})\Wv_L + \bv_L.
\end{equation}
Assuming that derivatives $d \xv/d t$ are available or can be computed, derivatives $d \zv/d t$ can also be computed:
\begin{align*}
  % \frac{d \zv}{d t} &= \ddt(\lv_{n-1})\Wv_n \\
  % &= \left(f'(\lv_{n-1}\Wv_{n-1} + \bv_{n-1}) \circ \left(\ddt \lv_{n-1}\Wv_{n-1}\right)\right)\Wv_n \\
  % &= \left(f'(\lv_{n-1}\Wv_{n-1} + \bv_{n-1}) \circ \left(\ddt \lv_{n-1}\Wv_{n-1}\right)\right)\Wv_n 
  \frac{d \zv}{d t} &= \left(f'(\lv_{L-1})\circ \frac{d \lv_{L-1}}{d t}\right)\Wv_L
  % &= \left( f'(\lv_{n-1}) \circ \left( \left(f'(\lv_{n-2}) \circ \ddt\lv_{n-2}\right)\Wv_{n-1}\right) \right)\Wv_n \\
  % &= \left( f'(\lv_{n-1}) \circ \left( \cdots \left( f'(\lv_0) \circ \frac{\dd \xv}{\dd t} \Wv_0 \right) \cdots \Wv_{n-1} \right)\right) \Wv_n.
\end{align*}
with
\begin{align*}
  \frac{d \lv_j}{d t} &= \left( f'(\lv_{j-1}) \circ \frac{d \lv_{j-1}}{d t}\right)\Wv_j \\
  \frac{d \lv_0}{d t} &= \frac{d \xv}{d t}\Wv_0.
\end{align*}
For the nonlinear pendulum example, we use a second order SINDy model that requires the calculation of second derivatives. Second derivatives can be computed using the following:
\begin{align*}
  \frac{d^2 \zv}{dt^2} &= \left(  f''(\lv_{L-1}) \circ \frac{d \lv_{L-1}}{dt} \circ \frac{d \lv_{L-1}}{dt} + f'(\lv_{L-1}) \circ \frac{d^2 \lv_{L-1}}{dt^2} \right)\Wv_L \\
  \frac{d^2 \lv_j}{dt^2} &= \left(  f''(\lv_{j-1})\circ \frac{d \lv_{j-1}}{dt} \circ \frac{d\lv_{j-1}}{dt} + f'(\lv_{j-1}) \circ \frac{d^2 \lv_{j-1}}{dt^2} \right)\Wv_j \\
  \frac{d\lv_0}{dt} &= \frac{d^2\xv}{dt^2}\Wv_0.
\end{align*}

\subsection{Training procedure}\label{sec:si_training}
We train multiple models for each of the example systems. Each instance of training has a different random initialization of the network weights. The weight matrices $\Wv_j$ are initialized using the Xavier initialization: the entries are chosen from a random uniform distribution over $[-\sqrt{6/\alpha},\sqrt{6/\alpha}]$ where $\alpha$ is the dimension of the input plus the dimension of the output \cite{glorot2010understanding}. The bias vectors $\bv_j$ are initialized to 0 and the SINDy model coefficients $\Xiv$ are initialized so that every entry is 1. We train each model using the Adam optimizer for a fixed number of epochs \cite{DBLP:journals/corr/KingmaB14}. The learning rate and number of training epochs for each example are specified in Section~\ref{sec:si_results}.

To obtain parsimonious dynamical models, we use a sequential thresholding procedure that promotes sparsity on the coefficients in $\Xiv$, which represent the dynamics on the latent variables ${\bf z}$. Every 500 epochs, we set all coefficients in $\Xiv$ with a magnitude of less than $0.1$ to 0, effectively removing these terms from the SINDy model. This is achieved by using a mask $\Upsilonv$, consisting of 1s and 0s, that determines which terms remain in the SINDy model. Thus the true SINDy terms in the loss function are given by
\begin{equation}
  \lambda_1 \frac{1}{m} \sum_{i=1}^m \left\|\dot{\xv}_i - \left(\nabla_\zv\psi(\varphi(\xv_i))\right)\left(\Thetav(\varphi(\xv_i)^T)(\Upsilonv \circ \Xiv)\right)\right\|_2^2 + \lambda_2 \frac{1}{m} \sum_{i=1}^m \left\|\nabla_\xv\varphi(\xv_i)\dot{\xv}_i - \Thetav(\varphi(\xv_i)^T)(\Upsilonv \circ \Xiv)\right\|_2^2
\end{equation}
where $\Upsilonv$ is passed in separately and not updated by the optimization algorithm. Once a term has been thresholded out during training, it is permanently removed from the SINDy model. Therefore the number of active terms in the SINDy model can only be decreased as training continues. The $L_1$ regularization on $\Xiv$ encourages the model coefficients to decrease in magnitude, which combined with the sequential thresholding produces a parsimonious dynamical model.

While the $L_1$ regularization penalty on $\Xiv$ promotes sparsity in the resulting SINDy model, it also encourages nonzero terms to have smaller magnitudes. This results in a trade-off between accurately reconstructing the dynamics of the system and reducing the magnitude of the SINDy coefficients, where the trade-off is determined by the relative magnitudes of the loss weight penalties $\lambda_1,\lambda_2$ and the regularization penalty $\lambda_3$. The specified training procedure therefore typically results in models with coefficients that are slightly smaller in magnitude than those which would best reproduce the dynamics. To account for this, we add an additional coefficient refinement period to the training procedure. To perform this refinement, we lock in the sparsity pattern in the dynamics by fixing the coefficient mask $\Upsilonv$ and continue training for 1000 epochs without the $L_1$ regularization on $\Xiv$. This ensures that the best coefficients are found for the resulting SINDy model and also allows the training procedure to refine the encoder and decoder parameters. This procedure is analagous to running a debiased regression following the use of LASSO to select model terms \cite{tibshirani2015statistical}.

\subsection{Model selection}\label{sec:si_model_selection}
Random initialization of the NN weights is standard practice for deep learning approaches. This results in the discovery of different models for different instances of training, which necessitates comparison among multiple models. In this work, when considering the success of a resulting model, one must consider the parsimony of the SINDy model, how well the decoder reconstructs the input, and how well the SINDy model captures the dynamics.

To assess model performance, we calculate the fraction of unexplained variance of both the input data $\xv$ and its derivative $\dot{\xv}$. This error calculation takes into account both the decoder reconstruction and the fit of the dynamics. When considering parsimony, we consider the number of active terms in the resulting SINDy model. While parsimonious models are desirable for ease of analysis and interpretability, a model that is too parsimonious may be unable to fully capture the dynamics. In general, for the examples explored, we find that models with fewer active terms perform better on validation data (lower fraction of unexplained variance of $\dot{\xv}$) whereas models with more active terms tend to over-fit the training data. %Models with too few active terms tend to have very poor prediction of the dynamics.

For each example system, we apply the training procedure to ten different initializations of the network and compare the resulting models. For the purpose of demonstration, for each example we show results for a chosen ``best'' model, which is taken to be the model with the lowest fraction of variance unexplained on validation data among models with the fewest active coefficients. While every instance of training does not result in the exact same SINDy sparsity pattern, the network tends to discover a few different closely related forms of the dynamics. We discuss the comparison among models for each particular example further in Section~\ref{sec:si_results}.

\section{Example Systems}\label{sec:si_results}

\subsection{Chaotic Lorenz system}\label{sec:si_lorenz}

\begin{figure*}%[tbhp]
\centering
\includegraphics[width=\linewidth]{fig_lorenz_si.pdf}
% \begin{overpic}[width=17.8cm]{../figures/fig_lorenz_si.pdf}
% % \put(3.5,45){(a)}
% % \put(3.5,17.5){(b)}
% \end{overpic}
\caption{Comparison of two discovered models for the Lorenz example system. For both models we show the equations, SINDy coefficients $\Xiv$, attractors, and simulated dynamics for two models discovered by the SINDy autoencoder. (a) A model with 7 active terms. This model can be rewritten in the same form as the original Lorenz system using the variable transformation described in Section~\ref{sec:si_lorenz}. Simulation of the model produces an attractor with a two lobe structure and is able to reproduce the true trajectories of the dynamics  for some time before eventually diverging due to the chaotic nature of the system. (b) A model with 10 active terms. The model has more terms than the true Lorenz system, but has a slightly lower fraction of unexplained variance of $\xv,\dot{\xv}$ than the model in (a). Simulation shows that the dynamics also lie on an attractor with two lobes. The model can accurately predict the true dynamics over a similar duration as (a).}
\label{fig:lorenz_si}
\end{figure*}

\begin{table}%[tbhp]
\centering
\caption{Hyperparameter values for the Lorenz example}
\label{table:lorenz_params}
\begin{tabular}{|l|r|}\hline
\bf Parameter & \bf Value \\ \hline\hline
% \midrule
n & 128 \\
d & 3 \\
training samples & $5.12 \times 10^5$ \\
batch size & 8000 \\
activation function & sigmoid \\
encoder layer widths & $64,32$ \\
decoder layer widths & $32,64$ \\
learning rate & $10^{-3}$ \\
SINDy model order & 1 \\
SINDy library polynomial order & 3 \\
SINDy library includes sine & no \\
SINDy loss weight $\dot{\mathbf{x}}$, $\lambda_1$ & $10^{-4}$ \\
SINDy loss weight $\dot{\mathbf{z}}$, $\lambda_2$ & $0$ \\
SINDy regularization loss weight, $\lambda_3$ & $10^{-5}$\\ \hline
% \bottomrule
\end{tabular}
\end{table}

To create a high-dimensional data set with dynamics defined by the Lorenz system, we choose six spatial modes $\mathbf{u}_1,\dots,\mathbf{u}_6 \in \Rb^{128}$ and take
\begin{align*}
  \mathbf{x}(t) = \mathbf{u}_1 z_1(t) + \mathbf{u}_2 z_2(t) + \mathbf{u}_3 z_3(t) + \mathbf{u}_4 z_1(t)^3 + \mathbf{u}_5 z_2(t)^3 + \mathbf{u}_6 z_3(t)^3.
\end{align*}
where the dynamics of $\mathbf{z}$ are specified by the Lorenz equations
\begin{subequations}
\begin{align}
  \dot{z}_1 &= \sigma(z_2 - z_1) \\
  \dot{z}_2 &= z_1(\rho - z_3) - z_2 \\
  \dot{z}_3 &= z_1 z_2 - \beta z_3
\end{align}
\label{eq:si_lorenz}
\end{subequations}
with standard parameter values of $\sigma=10, \rho=28,\beta=8/3$. We choose our spatial modes $\mathbf{u}_1,\dots,\mathbf{u}_6$ to be the first six Legendre polynomials defined at 128 grid points on a 1D spatial domain $[-1,1]$. To generate our data set, we simulate the system from 2048 initial conditions for the training set, 20 for the validation set, and 100 for the test set. For each initial condition we integrate the system forward in time from $t=0$ to $t=5$ with a spacing of $\Delta t=0.02$ to obtain $250$ samples. Initial conditions are chosen randomly from a uniform distribution over $z_1 \in [-36,36]$, $z_2 \in [-48,48]$, $z_3 \in [-16,66]$. This results in a training set with 512,000 total samples.

Following the training procedure described in Section~\ref{sec:si_training}, we learn ten models using the single set of training data (variability among the models comes from the initialization of the network weights). The hyperparameters used for training are shown in Table~\ref{table:lorenz_params}. For each model we run the training procedure for $10^4$ epochs, followed by a refinement period of $10^3$ epochs. Of the ten models, two have 7 active terms, two have 10 active terms, one has 11 active terms, and five have 15 or more active terms. While all models have less than 1\% unexplained variance for both $\xv$ and $\dot{\xv}$, the three models with 20 or more active terms have the worst performance  predicting $\dot{\xv}$. The two models with 10 active terms have the lowest overall error, followed by models with 7, 15, and 18 active terms. While the models with 10 active terms have a lower overall error than the models with 7 terms, both have a very low error and thus we choose to highlight the model with the fewest active terms. A model with 10 active terms is shown in Figure~\ref{fig:lorenz_si} for comparison.

For analysis, we highlight the model with the lowest error among the models with the fewest active terms. The discovered model has equations
\begin{subequations}
\begin{align}
  \dot{z}_1 &= -10.0 z_1 - 10.9 z_2 \\
  \dot{z}_2 &= - 0.9 z_2 + 9.6 z_1 z_3 \\
  \dot{z}_3 &= -7.1 - 2.7 z_3 - 3.1 z_1 z_2.
\end{align}
\end{subequations}
While the structure of this model appears to be different from that of the original Lorenz system, we can define an affine transformation that gives it the same structure. The variable transformation $z_1 = \alpha_1 \tilde{z}_1$, $z_2 = \alpha_2 \tilde{z}_2$, $z_3 = \alpha_3 \tilde{z}_3 + \beta_3$ gives the following transformed system of equations:
\begin{subequations}
\begin{align}
  \dot{\tilde{z}}_1 &= \frac{1}{\alpha_1}\left(-10.0 \alpha_1 \tilde{z}_1 - 10.9 \alpha_2 \tilde{z}_2\right) \\
                    &= -10.0 \tilde{z}_1 - 10.9 \frac{\alpha_2}{\alpha_1}\tilde{z}_2 \\
  \dot{\tilde{z}}_2 &= \frac{1}{\alpha_2}\left(-0.9 \alpha_2 \tilde{z}_2 + 9.6 \alpha_1 \tilde{z}_1 (\alpha_3 \tilde{z}_3 + \beta_3)\right) \\
                    &= 9.6 \frac{\alpha_1}{\alpha_2}\beta_3\tilde{z}_1 - 0.9\tilde{z}_2 + 9.6 \frac{\alpha_1\alpha_3}{\alpha_2}\tilde{z}_1\tilde{z}_3 \\
  \dot{\tilde{z}}_3 &= \frac{1}{\alpha_3}\left(-7.1 - 2.7 (\alpha_3 \tilde{z}_3 + \beta_3) - 3.1 \alpha_1 \alpha_2 \tilde{z}_1\tilde{z}_2\right) \\
                    &= \frac{1}{\alpha_3}(-7.1 - 2.7 \beta_3) - 2.7 \tilde{z}_3 - 3.1 \frac{\alpha_1\alpha_2}{\alpha_3}\tilde{z}_1\tilde{z}_2.
\end{align}
\end{subequations}
By choosing $\alpha_1 = 1$, $\alpha_2 = -0.917$, $\alpha_3 = 0.524$, $\beta_3 = -2.665$, the system becomes
\begin{subequations}
\begin{align}
  \dot{\tilde{z}}_1 &= -10.0 \tilde{z}_1 + 10.0 \tilde{z}_2 \label{eq:lorenz_transformed1}\\
  \dot{\tilde{z}}_2 &= 27.7 \tilde{z}_1 - 0.9 \tilde{z}_2 - 5.5 \tilde{z}_1\tilde{z}_3 \label{eq:lorenz_transformed2}\\
  \dot{\tilde{z}}_3 &= -2.7 \tilde{z}_3 + 5.5 \tilde{z}_1\tilde{z}_2 \label{eq:lorenz_transformed3}.
\end{align}
\end{subequations}
% \begin{subequations}
% \begin{align}
%   \dot{\tilde{z}}_1 &= -10.0 \tilde{z}_1 + 10.9 \tilde{z}_2 \\
%   \dot{\tilde{z}}_2 &= 25.2 \tilde{z}_1 - 0.9 \tilde{z}_2 - 9.6 \alpha_3 \tilde{z}_1\tilde{z}_3\\
%   \dot{\tilde{z}}_3 &= -2.7 \tilde{z}_3 + \frac{3.1}{\alpha_3} \tilde{z}_1\tilde{z}_2
% \end{align}
% \end{subequations}
This has the same form as the original Lorenz equations with parameters that are close in value, apart from an arbitrary scaling that affects the magnitude of the coefficients of $\tilde{z}_1\tilde{z}_3$ in \eqref{eq:lorenz_transformed2} and $\tilde{z}_1\tilde{z}_2$ in \eqref{eq:lorenz_transformed3}. The attractor dynamics for this system are very similar to the original Lorenz attractor and are shown in Figure~\ref{fig:lorenz_detail}c.

The learning procedure discovers a dynamical model by fitting coefficients that predict the continuous-time derivatives of the variables in a dynamical system. Thus it is possible for the training procedure to discover a model with unstable dynamics or which is unable to predict the true dynamics through simulation. We assess the validity of the discovered models by simulating the dynamics of the discovered low-dimensional dynamical system. Simulation of the system shows that the system is stable with trajectories existing on an attractor very similar to the original Lorenz attractor. Additionally, the discovered system is able to predict the dynamics of the original system. The fourth panel in Figure~\ref{fig:lorenz_si}a shows the trajectories found by stepping the discovered model forward in time as compared with the values of $\zv$ obtained by mapping samples of the high-dimensional data through the encoder. Although this is done on a new initial condition, the trajectories match very closely up to $t=5$, which is the duration of trajectories contained in the training set. After that the trajectories diverge, but the predicted trajectories remain on an attractor. The Lorenz dynamics are chaotic, and thus slight differences in coefficients or initial conditions cause trajectories to diverge quickly. 

For comparison, in Figure~\ref{fig:lorenz_si}b we show a second model discovered by the training procedure. This model has 10 active terms, as compared with 7 in the true Lorenz system. While the model contains additional terms not present in the original system, the dynamics lie on an attractor with a similar two lobe structure. Additionally, the system is able to predict the dynamics through simulation. This model has a lower error on test data than the original 7 term model, with a fraction of unexplained variance of $2\times 10^{-6}$ for $\xv$, $6 \times 10^{-5}$ for $\dot{\xv}$, and $3 \times 10^{-4}$ for $\dot{\zv}$.

\subsection{Reaction-diffusion}\label{sec:si_rd}

\begin{figure*}%[tbhp]
\centering
\begin{overpic}[width=11.4cm]{fig_rd.pdf}
  % \put(5,85){(a)}
  % \put(3,50){(b)}
  % \put(3,22){(c)}
\end{overpic}
\caption{Resulting models for the reaction-diffusion system. (a) Snapshots of the high-dimensional system show a spiral wave formation. (b,c) Equations, SINDy coefficients $\Xiv$, attractors, and simulated dynamics for two models discovered by the SINDy autoencoder. The model in (b) is a linear oscillation, whereas the model in (c) is a nonlinear oscillation. Both models achieve similar error levels and can predict the dynamics in the test set via simulation of the low-dimensional dynamical system.}
\label{fig:rd_detail}
\end{figure*}

\begin{table}%[tbhp]
\centering
\caption{Hyperparameter values for the reaction-diffusion example}
\label{table:rd_params}
\begin{tabular}{|l|r|}\hline
\bf Parameter & \bf Value \\\hline\hline
% \midrule
n & $10^4$ \\
d & 2 \\
training samples & 8000 \\
batch size & 1024 \\
activation function & sigmoid \\
encoder layer widths & $256$ \\
decoder layer widths & $256$ \\
learning rate & $10^{-3}$ \\
SINDy model order & 1 \\
SINDy library polynomial order & 3 \\
SINDy library includes sine & yes \\
SINDy loss weight $\dot{\mathbf{x}}$, $\lambda_1$ & $0.5$ \\
SINDy loss weight $\dot{\mathbf{z}}$, $\lambda_2$ & $0.01$ \\
SINDy regularization loss weight, $\lambda_3$ & $0.1$\\ \hline
% \bottomrule
\end{tabular}
\end{table}

We generate data from a high-dimensional lambda-omega reaction-diffusion system governed by
\begin{subequations}
\begin{align}
  u_t &= (1-(u^2+v^2))u + \beta (u^2+v^2) v + d_1 (u_{xx} + u_{yy}) \\
  v_t &= -\beta (u^2+v^2)u + (1-(u^2+v^2))v + d_2 (v_{xx} + v_{yy})
\end{align}
\end{subequations}
with $d_1,d_2=0.1$ and $\beta=1$. The system is simulated from a single initial condition from $t=0$ to $t=10$ with a spacing of $\Delta t=0.05$ for a total of 10,000 samples. The initial condition is defined as
\begin{subequations}
\begin{align}
  u(y_1,y_2,0) &= \tanh\left(\sqrt{y_1^2 + y_2^2}\cos\left(\angle(y_1+iy_2) - \sqrt{y_1^2 + y_2^2}\right)\right) \\
  v(y_1,y_2,0) &= \tanh\left(\sqrt{y_1^2 + y_2^2}\sin\left(\angle(y_1+iy_2) - \sqrt{y_1^2 + y_2^2}\right)\right)
\end{align}
\end{subequations}
over a spatial domain of $y_1 \in [-10,10],\ y_2\in[-10,10]$ discretized on a grid with 100 points on each spatial axis. The solution of these equations results in a spiral wave formation. We apply our method to snapshots of $u(y_1,y_2,t)$ generated by the above equations, multiplied by a Gaussian $f(y_1,y_2) = \exp(-0.1(y_1^2+y_2^2))$ centered at the origin to localize the spiral wave in the center of the domain. Our input data is thus defined as $\xv(t) = f(:,:) \circ u(:,:,t) \in \Rb^{10^4}$. We also add Gaussian noise with a standard deviation of $10^{-6}$ to both $\xv$ and $\dot{\xv}$. Four time snapshots of the input data are shown in Figure~\ref{fig:rd_detail}a.

We divide the total number of samples into training, validation, and test sets: the last 1000 samples are taken as the test set, 1000 samples are chosen randomly from the first 9000 samples as a validation set, and the remaining 8000 samples are taken as the training set. We train ten models using the procedure outlined in Section~\ref{sec:si_training} for $3 \times 10^3$ epochs followed by a refinement period of $10^3$ epochs. Hyperparameters used for training are shown in Table~\ref{table:rd_params}. Nine of the ten resulting dynamical systems models have two active terms and one has three active terms. The dynamical equations, SINDy coefficient matrix, attractors, and simulated dynamics for two example models are shown in Figure~\ref{fig:rd_detail}b,c. The models with two active terms all have one of the two forms shown in the figure: three models have a linear oscillation and six models have a nonlinear oscillation. Both model forms have similar levels of error on the test set and are able to predict the dynamics in the test set from simulation, as shown in the fourth panel of Figure~\ref{fig:rd_detail}b,c.

\subsection{Nonlinear pendulum}\label{sec:si_pendulum}

\begin{figure*}%[tbhp]
\centering
\begin{overpic}[width=\linewidth]{fig_pendulum.pdf}
  % % equations - true
  % \put(15,30){$\ddot{z} = -\sin z$}
  % % equations - discovered
  % \put(15,15){$\ddot{z} = -1.15 \sin z$}
  % % coefficient matrix labels
  % \put(45.5,30.5){\small $1$}
  % \put(45,28){\small $z$}
  % \put(45,25){\small $\dot{z}$}
  % \put(45,21.5){\small $z^2$}
  % \put(46,15){$\vdots$}
  % \put(45,8){\small $z_2^3$}
  % \put(41,5){\small $\sin z$}
  % \put(41,1.5){\small $\sin \dot{z}$}
  % % attractor labels
  % \put(59,20){$z_2$}
  % \put(68,12){$z_1$}
  % % dynamics labels
  % \put(78,23.5){$z_2$}
  % \put(78,14){$z_1$}
\end{overpic}
\caption{Resulting models for the nonlinear pendulum. (a) Snapshots of the high-dimensional system are images representing the position of the pendulum in time. (b,c,d) Comparison of two discovered models with the true pendulum dynamics. Equations, SINDy coefficients $\Xiv$, attractors, and simulated dynamics for the true pendulum equation are shown in (b). The model in (c) correctly discovered the true form of the pendulum dynamics. Both the image of the attractor and simulations match the true dynamics. (d) In one instance of training, the SINDy autoencoder discovered a linear oscillation for the dynamics. This model achieves a worse error than the model in (c).}
\label{fig:pendulum_detail}
\end{figure*}

\begin{table}%[tbhp]
\centering
\caption{Hyperparameter values for the nonlinear pendulum example}
\label{table:pendulum_params}
\begin{tabular}{|l|r|}\hline
\bf Parameter & \bf Value \\\hline\hline
% \midrule
n & $2601$ \\
d & 1 \\
training samples & $5 \times 10^4$\\
batch size & 1024 \\
activation function & sigmoid \\
encoder layer widths & $128,64,32$ \\
decoder layer widths & $32,64,128$ \\
learning rate & $10^{-4}$ \\
SINDy model order & 2 \\
SINDy library polynomial order & 3 \\
SINDy library includes sine & yes \\
SINDy loss weight $\dot{x}$, $\lambda_1$ & $5 \times 10^{-4}$ \\
SINDy loss weight $\dot{z}$, $\lambda_2$ & $5 \times 10^{-5}$ \\
SINDy regularization loss weight, $\lambda_3$ & $10^{-5}$\\\hline
% \bottomrule
\end{tabular}
\end{table}

The nonlinear pendulum equation is given by
\begin{equation}
  \ddot{z} = -\sin z. \label{eq:pendulum}
\end{equation}
We generate synthetic video of the pendulum in two spatial dimensions by creating high-dimensional snapshots given by
\begin{equation}
  x(y_1,y_2,t) = \exp\left(-\!20\!\left((y_1\! -\! \cos(z(t)\!-\!\pi/2))^2 + (y_2\! -\! \sin(z(t)\!-\!\pi/2))^2 \right) \right)
\end{equation}
at a discretization of $y_1,y_2\!\in\![-1.5,1.5]$. We use 51 grid points in each dimension resulting in snapshots $\xv(t) \in \Rb^{2601}$. To generate a training set, we simulate \eqref{eq:pendulum} from 100 randomly chosen initial conditions with $z(0) \in [-\pi,\pi]$ and $\dot{z}(0) \in [-2.1,2.1]$. The initial conditions are selected from a uniform distribution in the specified range but are restricted to conditions for which the pendulum does not have enough energy to do a full loop. This condition is determined by checking that $|\dot{z}(0)^2/2 - \cos z(0)| \leq 0.99$.

Following the training procedure outlined in Section~\ref{sec:si_training}, we train ten models for $5 \times 10^3$ epochs followed by a refinement period of $10^3$ epochs. Hyperparameters used for this example are shown in Table~\ref{table:pendulum_params}. Five of the ten resulting models correctly recover the nonlinear pendulum equation. These five models have the best performance of the ten models. The attractor and simulated dynamics for the best of these five models are shown in Figure~\ref{fig:pendulum_detail}. One model, also shown in Figure~\ref{fig:pendulum_detail}, recovers a linear oscillator. This model is able to achieve a reasonably low prediction error for $\ddot{\xv},\ddot{\zv}$ but the simulated dynamics, while still oscillatory, appear qualitatively different from the true pendulum dynamics. The four remaining models all have two active terms in the dynamics and have a worse performance than the models with one active term.
